# Supplementary material for: DecodingTrust: A Comprehensive Assessment of Trustworthiness in GPT Models
Source: arXiv:2306.11698 source file (2024-02-26)
Supplement: Supplementary file 7 [file fairness_short_appendix.tex]

\section{Additional details of evaluation on fairness}
\label{app:sec:fairness}
In this section, we study the fairness of GPT-3.5 and GPT-4 in different settings. In particular, we explore the dependence between the predictions of GPT models and sensitive attributes (e.g., sex and race) and whether there is a fairness gap between GPT-3.5 and GPT-4 in \Cref{app:sec:fairness_zero_shot}.
We then study the relationship between the fairness of the data distribution that the few-shot training examples are drawn from and the fairness of model predictions in \Cref{app:sec:fairness_few_shot_1}.
We further explore how the number of training examples in few-shot learning  affects the fairness of GPT models in \Cref{app:sec:fairness_few_shot_2}.

\subsection{Metrics of fairness}
\label{app:sec:fairness_metric}
We introduce the definitions of fairness metrics used to evaluate the fairness of model predictions and the fairness of the generated few-shot training sentences.
Suppose that we have $n$ data samples $\{(X,Y,A)\}_{i=1}^n$ with features $X \in \mathcal{X}$, labels $Y \in \mathcal{Y}:= \{0,1\}$, and a sensitive attribute $A \in \{0,1\}$ drawn from the distribution $P_{XY}$.
Note that the sensitive attribute $A$ is also included in the feature vector $X$. 
Let $f: \mathcal{X} \mapsto \mathcal{Y}$ represent a machine learning model. We adopt the metric of demographic parity difference $M_{\text{dpd}}$ in \cite{pmlr-v28-zemel13}: $M_{\text{dpd}} = \left| \mathbb{P}_{(X,Y,A)\sim P_{XY}}[f(X)=1 | A=1] -  \mathbb{P}_{(X,Y,A)\sim P_{XY}}[f(X)=1 | A=0] \right|$.

The \textbf{demographic parity difference} measures the difference between the probability of positive predictions conditioned on sensitive attribute $A=1$ and that conditioned on $A=0$.
A large demographic parity difference $M_{\text{dpd}}$ means that there is a large prediction gap between the groups with $A=1$ $A=0$, indicating the unfairness of the model prediction.
Since the demographic parity difference does not consider the ground truth label, we also consider the metric of \textbf{equalized odds difference} $M_{\text{eod}}$ in \cite{NIPS2016_9d268236}: $M_{\text{eod}} = \max \left\{ M_{TP}, M_{FP}  \right\}$, where $M_{TP}$ is the true positive equalized odds difference: $\small M_{TP} = \left| \mathbb{P}_{(X,Y,A)\sim P_{XY}}[f(X)=1 | Y=1, A=0] -  \mathbb{P}_{(X,Y,A)\sim P_{XY}}[f(X)=1 | Y=1, A=1] \right|$
and $M_{FP}$ is the false positive equalized odds difference:
$\small M_{FP} = \left| \mathbb{P}_{(X,Y,A)\sim P_{XY}}[f(X)=1 | Y=0, A=0] -  \mathbb{P}_{(X,Y,A)\sim P_{XY}}[f(X)=1 | Y=0, A=1] \right|$.
A large equalized odds difference $M_{\text{eod}}$ demonstrates a large prediction gap conditioned on different values of the sensitive attribute, and therefore indicates the unfairness of the model prediction.

To evaluate the fairness of the data distribution, we adopt the base rate parity $b_P$ for distribution $P$ in \cite{NEURIPS2019_b4189d9d,kang2022certifying}:
$b_P =  \mathbb{P}_{(X,Y,A)\sim P_{XY}}[Y=1 | A=1] -  \mathbb{P}_{(X,Y)\sim P_{XYA}}[Y=1 | A=0]$.
A large base rate parity $b_P$  shows the bias of the data distribution regarding different values of the sensitive attribute $A$, indicating that the data distribution $P$ is biased and unfair.
In the evaluation, we consider both the base rate parity of data distribution in the context of few-shot training examples $b_{P_c}$ and the base rate parity of the test set $b_{P_t}$. 

% \begin{figure}
%     \centering
%     \includegraphics[width=\linewidth]{figures/fairness_example.png}
%     \caption{\small Examples of fairness evaluation in the zero-shot and few-shot settings.
%      The \textcolor{ForestGreen}{green} dialogue box refers to the user input;
%     the \textcolor{Goldenrod}{yellow} dialogue box refers to user-provided example responses as few-shot demonstrations;
%     the \textcolor{magenta}{red} dialogue box refers to the real responses from GPT-3.5 and GPT-4. }
%     \label{app:fig:fairness}
% \end{figure}

\subsection{Fairness evaluation in zero-shot setting}
\label{app:sec:fairness_zero_shot}

In this part, we aim to explore \textit{(1) whether the predictions of GPT models are fair regarding different sensitive attributes, and (2) whether there is a fairness gap between the predictions of GPT-3.5 and GPT-4  in the zero-shot setting.}

\textbf{Evaluation setup.} We select a commonly used fairness evaluation dataset Adult~\cite{asuncion2007uci}, transform the tabular data into language descriptions, and ask GPT models to perform classification tasks on it.
The Adult dataset includes 14 attributes of a person (e.g., age and education level) as input. The task is to predict whether the income of the person is over \$$50$k per year. We evaluate the fairness of GPT models on multiple sensitive attributes, including sex, race, and age.
% Specifically, we have ``male'' and ``female'' for the attribute of sex, ``white'' and ``black'' for race, and ``above average'' and ``below average'' for age.
% % following the literature \cite{NEURIPS2020_55d491cf,NEURIPS2021_07563a3f}.
% One of the tabular data is: ```A person in 1996 has the following attributes: age: 19, workclass: private, final weight: 192773, education: HS-grad, highest education level: 9, marital status: never-married, occupation: other-service, relationship: own-child, race: white, sex: female, capital gain: 0, capital loss: 0, hours per week: 24, native country: United-States'''.
% An illustrative example of evaluations on GPT models is shown in \Cref{app:fig:fairness}.
To show whether there is a large performance gap across different groups regarding the sensitive attribute, we evaluate GPT models on the test set with different base rate parity $b_{P_t}$. 
We select 200 samples to construct the test set.

\textbf{Results.} \Cref{app:tab:fairness_adult_zero_shot} indicates that both GPT-3.5 and GPT-4 demonstrate fairness issues. 
The accuracy and unfairness scores (i.e., $M_{\text{dpd}}$ and $M_{\text{eod}}$) between the groups with sensitive attribute $A=0$ and $A=1$ increase significantly as the test set becomes less and less fair (i.e., a larger base rate parity $b_{P_t}$), indicating the tradeoff between accuracy and fairness.
% Specifically, with a large base rate parity $b_{P_t}$, the constructed test set is more biased towards $Y=1$ (e.g., high salary) conditioned on $A=1$ (e.g., male), and therefore a higher accuracy with a larger $b_{P_t}$ indicates the model's bias towards the group with $A=1$.
Furthermore, we find that GPT-4 consistently achieves higher unfairness scores than GPT-3.5, demonstrating the fairness issues of GPT-4.
We also evaluate the fairness of GPT models for different sensitive attributes, including sex, race, and age.
\Cref{app:tab:fairness_sensitive_attr} indicates that GPT-4 demonstrates more unfair predictions for different sensitive attributes, and the unfairness issues of GPT models are more severe for certain sensitive attributes such as sex and race.

% \textbf{Setting.} We similarly transform the tabular data in Adult dataset into language descriptions and ask GPT models to perform similar classification tasks. We select the sensitive attributes, such as sex (male and female), race (white and black), and age (below average and above average). We evaluate GPT models in zero-shot settings to demonstrate their intrinsic fairness for different sensitive attributes. We randomly select $200$ test samples with the constraint of base rate parity $b_{P_t}=0.0$ to avoid the bias induced by a skewed test set.

% \textbf{Result.} \Cref{app:tab:fairness_sensitive_attr} indicates that 1) GPT-4 demonstrates more unfair predictions for different sensitive attributes, and 2) the unfairness issues of GPT models are more severe for certain sensitive attributes such as sex and race.

\begin{table}[t]\small
    \centering
    \caption{\small Accuracy (ACC (\%)), demographic parity difference ($M_{\text{dpd}}$), and equalized odds difference ($M_{\text{eod}}$) on Adult test set with different base rate parity $b_{P_t}$ in zero-shot setting.}
       \resizebox{0.8\linewidth}{!}{
    \begin{tabular}{c|ccc|ccc|ccc}
    \toprule
    \multirow{2}{*}{Model}    &  \multicolumn{3}{c}{$b_{P_t}=0.0$}  &  \multicolumn{3}{c}{$b_{P_t}=0.5$}  &  \multicolumn{3}{c}{$b_{P_t}=1.0$} \\
        & ACC $\uparrow$ & $M_{\text{dpd}}$ $\downarrow$  & $M_{\text{eod}}$ $\downarrow$   & ACC $\uparrow$ & $M_{\text{dpd}}$ $\downarrow$  & $M_{\text{eod}}$ $\downarrow$   & ACC $\uparrow$ & $M_{\text{dpd}}$ $\downarrow$ & $M_{\text{eod}}$ $\downarrow$ \\
    \midrule
     GPT-3.5   & 63.5 & \textbf{0.17} & \textbf{0.20} & 68.5 & \textbf{0.31} & \textbf{0.19} & 73.0 & \textbf{0.46} & \textbf{0.49} \\
     GPT-4   & \textbf{72.5} & 0.21 & 0.26 & \textbf{78.5} & 0.47 & 0.40 & \textbf{85.5} & 0.71 & 0.95 \\
    \bottomrule
    \end{tabular}
    }
    \label{app:tab:fairness_adult_zero_shot}
\end{table}

\begin{table}[t]\small
    \centering
    \caption{\small Demographic parity difference ($M_{\text{dpd}}$) and equalized odds difference ($M_{\text{eod}}$)  with different sensitive attributes on Adult dataset with test base rate parity $b_{P_t}=0.0$ in the zero-shot setting. }
    \resizebox{0.6\linewidth}{!}{
     \begin{tabular}{c|cc|cc|cc}
    \toprule
    \multirow{2}{*}{Model}    &  \multicolumn{2}{c}{Sex}  &  \multicolumn{2}{c}{Race}  &  \multicolumn{2}{c}{Age} \\
       & $M_{\text{dpd}}$ $\downarrow$  & $M_{\text{eod}}$ $\downarrow$  & $M_{\text{dpd}}$ $\downarrow$  & $M_{\text{eod}}$ $\downarrow$  & $M_{\text{dpd}}$ $\downarrow$ & $M_{\text{eod}}$ $\downarrow$ \\
    \midrule
     GPT-3.5   & \textbf{0.17} & \textbf{0.20} & \textbf{0.14} & \textbf{0.17} & \textbf{0.09}  & \textbf{0.15}  \\
     GPT-4   & 0.21 & 0.26 & 0.16 & 0.28 & 0.14 &  0.20 \\
    \bottomrule
    \end{tabular}
    }
    \label{app:tab:fairness_sensitive_attr}
\end{table}

\subsection{Fairness evaluation under unfair context in few-shot setting}
\label{app:sec:fairness_few_shot_1}

In this part, we aim to explore whether the fairness of model predictions is affected by the fairness of context provided by the few-shot examples. 

\textbf{Evaluation setup.} We similarly transform the tabular data in Adult ~\cite{asuncion2007uci} into language descriptions and ask GPT models to perform the classification tasks. The sensitive attribute sex is selected, and $A=0$ denotes female and $A=1$ denotes male.
We consider 32 fwe-shot training instances here since it is the maximum number of examples we can have given the token number limitation of GPT models.
We construct three contexts based on different fairness levels with base rate parity $b_{P_c}=0.0,0.5,1.0$.
A large base rate parity $b_{P_c}$ indicates the bias towards a positive prediction $Y=1$ (i.e., high salary) conditioned on $A=1$ (i.e., male) over $A=0$ (i.e., female). 
Similarly, we sample 200 samples as the test set. We fix the base rate parity of the test set $b_{P_t}$ as $0.0$ to demonstrate the unfairness induced from the training context.

\textbf{Results.} \Cref{app:tab:fairness_adult_few_shot_1} shows that when the training context is less fair (i.e., a larger base rate parity $b_{P_c}$), the predictions of GPT models also become less fair (i.e., larger $M_{\text{dpd}}$  and $M_{\text{eod}}$ ). 
We find that only $32$ samples with group bias in the context can affect the fairness of GPT model predictions very effectively. 
The demographic parity difference $M_{\text{dpd}}$ of GPT-3.5 is increased from $0.033$ to $0.12$, and that of GPT-4.0 is increased from $0.10$ to $0.28$. 
This conclusion also holds for the metric of equalized odds difference $M_{\text{eod}}$.

\begin{table}[t]\small
    \centering
    \caption{Accuracy (ACC (\%)), demographic parity difference ($M_{\text{dpd}}$), and equalized odds difference ($M_{\text{eod}}$) on Adult dataset using demonstrations with different base rate parity $b_{P_c}$ in the 32-shot learning. The base rate parity of the test set $b_{P_t}$ is fixed as $0.0$ to demonstrate the unfairness induced by the context.}
       \resizebox{0.8\linewidth}{!}{
    \begin{tabular}{c|ccc|ccc|ccc}
    \toprule
    \multirow{2}{*}{Model}   &  \multicolumn{3}{c}{$b_{P_c}=0.0$}  &  \multicolumn{3}{c}{$b_{P_c}=0.5$}  &  \multicolumn{3}{c}{$b_{P_c}=1.0$} \\
       & ACC $\uparrow$ & $M_{\text{dpd}}$ $\downarrow$  & $M_{\text{eod}}$ $\downarrow$   & ACC $\uparrow$ & $M_{\text{dpd}}$ $\downarrow$  & $M_{\text{eod}}$ $\downarrow$   & ACC $\uparrow$ & $M_{\text{dpd}}$ $\downarrow$ & $M_{\text{eod}}$ $\downarrow$ \\
    \midrule
     GPT-3.5   & 61.5 & \textbf{0.033} & \textbf{0.057} & 69.5 & \textbf{0.026} & \textbf{0.062} & 70.5 & \textbf{0.12} & \textbf{0.20} \\
     GPT-4   & \textbf{72.0} & 0.10 & 0.12 & \textbf{78.5} & 0.11 & 0.14 & \textbf{79.0} & 0.28 & 0.34 \\
    \bottomrule
    \end{tabular}
    }
    \label{app:tab:fairness_adult_few_shot_1}
\end{table}

\subsection{Fairness evaluation given fair context}
\label{app:sec:fairness_few_shot_2}

In this part, we aim to explore how the fairness of model predictions are affected by the number of few-shots.

\textbf{Evaluation setup.} 
We similarly transform the tabular data in Adult dataset into language descriptions and ask GPT models to perform classification tasks. The sensitive attribute is selected as sex, and $A=0$ denotes female and $A=1$ denotes male. We randomly select $200$ test samples with the constraint of base rate parity $b_{P_t}=0.5$ for fair comparisons across evaluations with different numbers of few-shot examples.
We perform the evaluation with $0,16,32$ few-shot instances with base rate parity $b_{P_c}=0$.
In other words, we want to study whether the predictions of GPT models become more fair given more examples in a fair context. 

\textbf{Results.} \Cref{app:tab:fairness_adult_few_shot_2} indicates that with a larger number of few-shots training examples in the fair context, the accuracy of GPT models decreases given biased test sets, and the model predictions become fairer.
The observation demonstrates that the bias of GPT models towards certain groups can be reduced by adding fair and balanced few-shot training examples, which is aligned with the previous finding on GPT-3 \cite{si2023prompting}.
Moreover, a fair context involving only 16 instances is already effective in guiding the predictions of GPT models to be fairer.
Note that the prediction accuracy of GPT models is decreased with more fair demonstrations.

\begin{table}[t]\small
    \centering
    \caption{\small Accuracy (ACC (\%)), demographic parity difference ($M_{\text{dpd}}$), and equalized odds difference ($M_{\text{eod}}$) on Adult dataset with different \#shot in the in-context learning. The base rate parity of the demonstrations $b_{P_c}$ is fixed as $0.0$, and the base rate parity of the test set is fixed as $0.5$.}
       \resizebox{0.8\linewidth}{!}{
    \begin{tabular}{c|ccc|ccc|ccc}
    \toprule
    \multirow{2}{*}{Model}    &  \multicolumn{3}{c|}{\# shot = 0}  &  \multicolumn{3}{c|}{\# shot = 16}  &  \multicolumn{3}{c}{\# shot = 32} \\
       & ACC $\uparrow$ & $M_{\text{dpd}}$ $\downarrow$  & $M_{\text{eod}}$ $\downarrow$   & ACC $\uparrow$ & $M_{\text{dpd}}$ $\downarrow$  & $M_{\text{eod}}$ $\downarrow$   & ACC $\uparrow$ & $M_{\text{dpd}}$ $\downarrow$ & $M_{\text{eod}}$ $\downarrow$ \\
    \midrule
     GPT-3.5   &  73.0 & \textbf{0.46} & \textbf{0.49} & 67.5 & \textbf{0.25} & \textbf{0.084} & 63.5 & \textbf{0.19} & \textbf{0.10} \\
     GPT-4   &  \textbf{85.5} & 0.71 & 0.95 & \textbf{78.0} & 0.38 & 0.27 & \textbf{75.0} & 0.30 & 0.13\\
    \bottomrule
    \end{tabular}
    }
    \label{app:tab:fairness_adult_few_shot_2}
\end{table}

\begin{takeaway}[Takeaways]
\begin{itemize}[leftmargin=1.3em,topsep=1pt,noitemsep]
    \item GPT-4 is more accurate than GPT-3.5 for prediction, while GPT-3.5 is fairer than GPT-4 in different settings, indicating the accuracy-fairness tradeoffs.
    \item In the zero-shot setting, both GPT-3.5 and GPT-4 have large performance gaps across groups with different levels of bias considering different sensitive attributes, indicating that GPT models are intrinsically biased to certain groups.
    \item In the few-shot setting, the performance of both GPT-3.5 and GPT-4 are influenced by the base rate parity (fairness) of the constructed few-shot demonstrations. Less fair demonstrations will induce more biased predictions for GPT models. 
    \item The bias of GPT models can be reduced by providing a fair training context. Fair training context involving only a few fair demonstrations (e.g., 16 samples on Adult dataset) can effectively guide GPT models to be fairer.
    \end{itemize}
\end{takeaway}
